# Supplementary material for: Kernel-based Distance Metric Learning in the Output Space
Source: arXiv:1312.2578 source file (2014-04-28)
Supplement: Supplementary file 1 [file Appendix.tex]

\section*{Supplementary Material}

% Reset all acronyms
\acresetall
